# Supplementary material for: Beyond Pixels: Visual Metaphor Transfer via Schema-Driven Agentic Reasoning
Source: arXiv:2602.01335 source file (2026-08-27)
Supplement: Supplementary file 1 [file supp1.tex]

\begin{figure*}[h]
  \centering
  \includegraphics[width=0.85\linewidth]{sup/Images/supp1.pdf}
  \caption{\textbf{Additional results of our method.}}
  \label{fig:supp1}
\end{figure*}
